# Supplementary material for: FedQV: Leveraging Quadratic Voting in Federated Learning
Source: arXiv:2401.01168 source file (2024-04-09)
Supplement: Supplementary file 1 [file appendix_rebuttal.tex]

\section{Results}

\begin{figure}[!htbp]
  \centering
 \begin{subfigure}[b]{0.3\textwidth}
    \includegraphics[width=\linewidth]{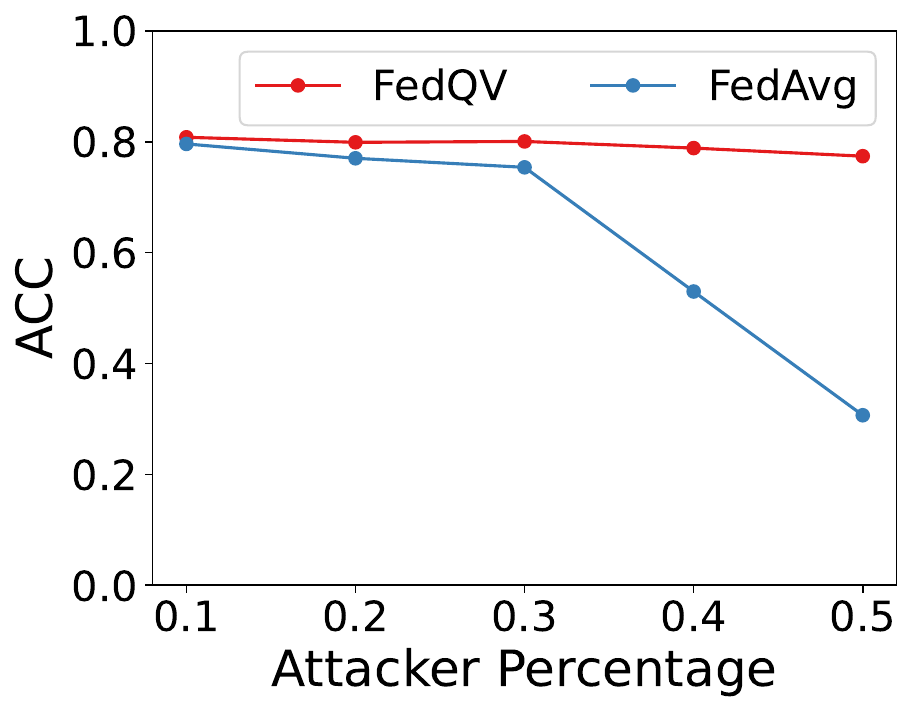}
    \caption{Under the Min-Max Attack }
    \label{fig:FEMNIST_min_max}
  \end{subfigure}
  \hfill
  \begin{subfigure}[b]{0.3\textwidth}
    \includegraphics[width=\linewidth]{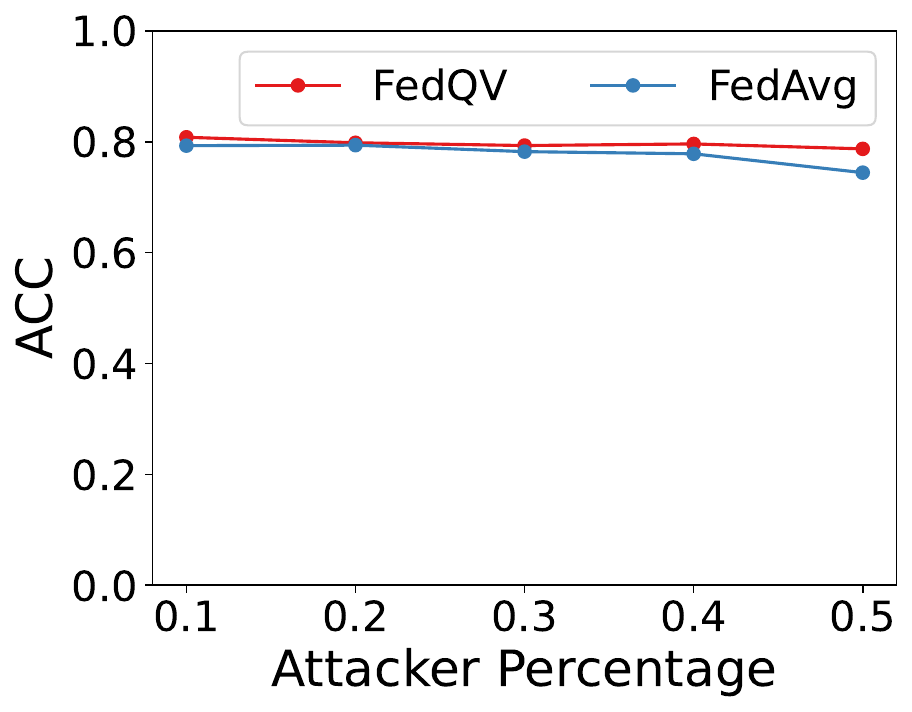}
    \caption{Under Min-Sum Attack}
\label{fig:FEMNIST_min_sum}
  \end{subfigure}
  \hfill
  \begin{subfigure}[b]{0.3\textwidth}
    \includegraphics[width=\linewidth]{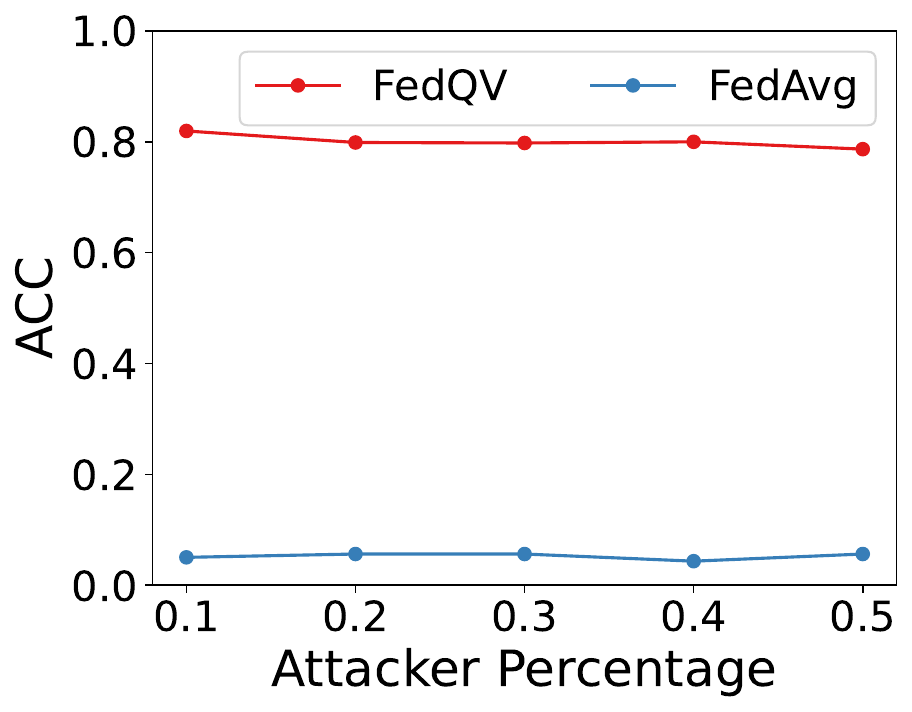}
    \caption{Under QV Adaptive Attack} \label{fig:FEMNIST_adaptive}
  \end{subfigure}
  
  \caption{Comparison of Accuracy (ACC) for \textsc{FedQV} and \textsc{FedAvg} over 100 epochs on FEMNIST datasets under various model poisoning attacks, with varying percentages of attackers from 10\% to 50\%.}
  \label{fig:three_subfigures}
\end{figure}


\begin{figure}[htbp]
  \centering
  \begin{subfigure}[b]{0.48\textwidth}
    \includegraphics[width=\linewidth]{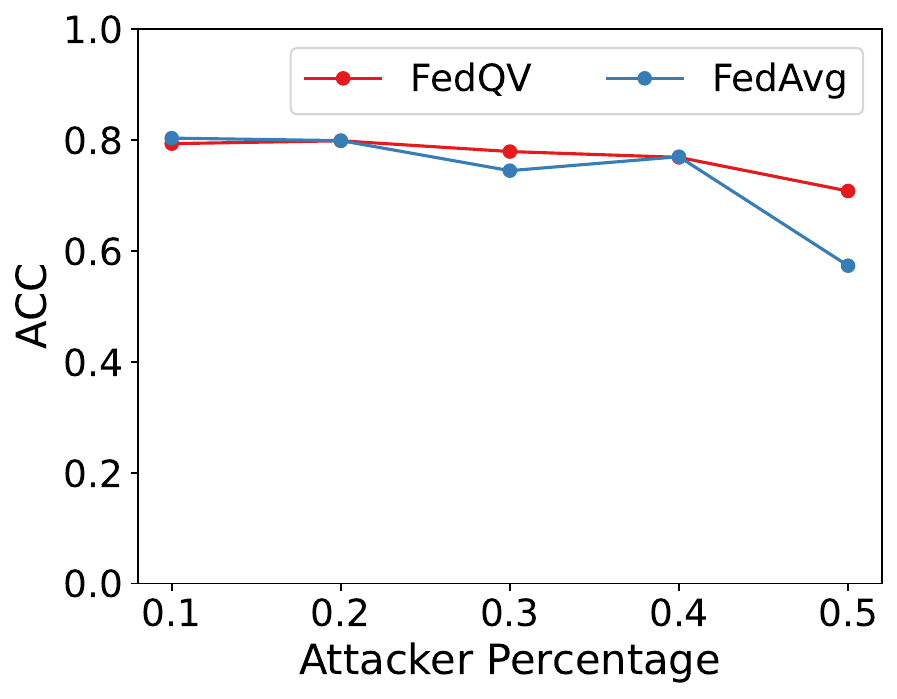}
    \caption{Accuracy(ACC) Metric}
    \label{fig:FEMNIST_neuro_acc}
  \end{subfigure}
  \hfill
  \begin{subfigure}[b]{0.48\textwidth}
    \includegraphics[width=\linewidth]{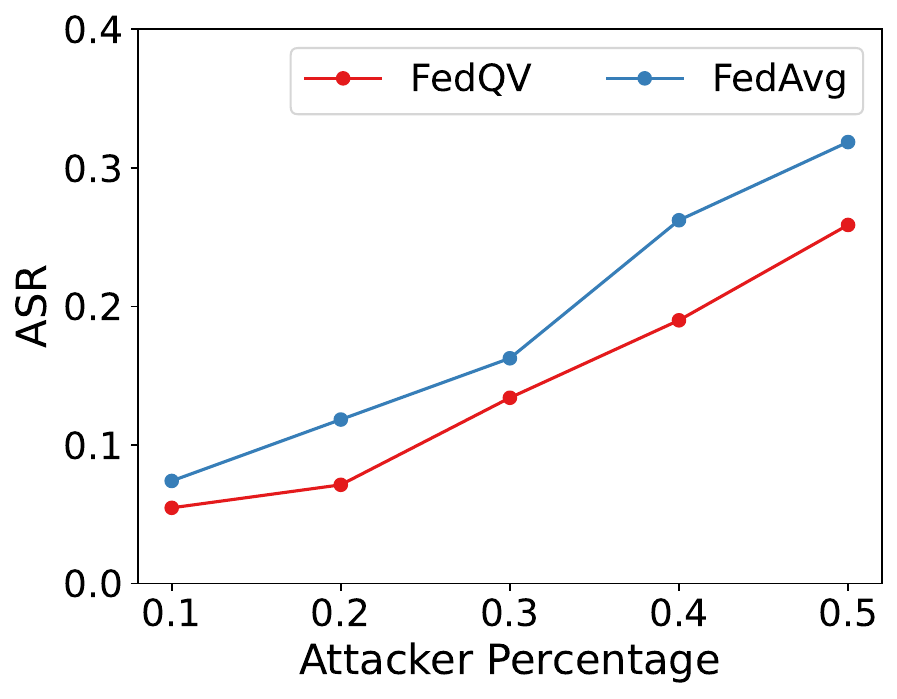}
    \caption{Attack Success Rate (ASR) Metric}
    \label{fig:FEMNIST_neuro_asr}
  \end{subfigure}
  
  \caption{Comparison of Accuracy (ACC) and Attack Success Rate (ASR) for \textsc{FedQV} and \textsc{FedAvg} under Neurotoxin Attack over 100 epochs on FEMNIST Dataset, with varying percentages of attackers from 10\% to 50\%.}
  \label{fig:FEMNIST_neuro}
\end{figure}

\begin{table}[!htbp]
\centering
\begin{tabular}{@{}rlllll@{}}
\toprule
\multicolumn{6}{c}{Fashion-MNIST}                                                                                                                  \\ \midrule
\multicolumn{1}{c}{Non-IID} & \multicolumn{1}{c}{0.1} & \multicolumn{1}{c}{0.3} & \multicolumn{1}{c}{0.5} & \multicolumn{1}{c}{0.7} & \multicolumn{1}{c}{0.9} \\ \cmidrule(l){2-6} 
FedQV  &                           &                           &                           &                           &                           \\
ACC    & \multicolumn{1}{r}{84.94} & \multicolumn{1}{r}{86.01} & \multicolumn{1}{c}{83.88} & \multicolumn{1}{c}{81.37} & \multicolumn{1}{r}{75.96} \\
ASR    & \multicolumn{1}{r}{3.39}  & 4.55                      & 17.64                     & 20.59                     & \multicolumn{1}{r}{24.18} \\
FedAvg &                           &                           &                           &                           &                           \\
ACC    & 81.27                     & 81.1                      & 82.44                     & \multicolumn{1}{r}{80.77} & 65.68                     \\
ASR    & \multicolumn{1}{c}{3.37}  & \multicolumn{1}{c}{13.39} & \multicolumn{1}{c}{20.84} & \multicolumn{1}{c}{22.99} & \multicolumn{1}{c}{60.35} \\ \bottomrule
\end{tabular}
\vspace{3mm}
\caption{Comparison of Accuracy (ACC) and Attack Success Rate (ASR) for FedQV and FedAvg under Backdoor Attack over 100 epochs with varying Non-IID Degrees on Fashion-MNIST Dataset.}
\label{tab:non-iid}
\end{table}
